# Supplementary material for: Low-Rank Knowledge Decomposition for Medical Foundation Models
Source: arXiv:2404.17184 source file (2024-04-26)
Supplement: Supplementary file 1 [file X_suppl.tex]

\clearpage
\setcounter{page}{1}
\maketitlesupplementary

\section{Detailed Introduction of Datasets}
\begin{itemize}
    \item Radimagenet consists 1.35 million images and we decompose its publicly released pre-trained model into 11  lightweight expert models based on anatomic regions. 
    \item MedMnist-sub consists of a total of 705,689 images from MedMnistV2 and we decomposed its pre-trained model into 10 lightweight expert models based on anatomic regions.
    \item Med-ML is a custom dataset we constructed, which contains a total of 119,655 images, and we decomposed the model pre-trained on it into 8 lightweight expert models based on tasks.
\end{itemize}

\begin{figure*}[h]
\begin{minipage}{0.48\linewidth}
 \centerline{\includegraphics[width=0.98\linewidth]{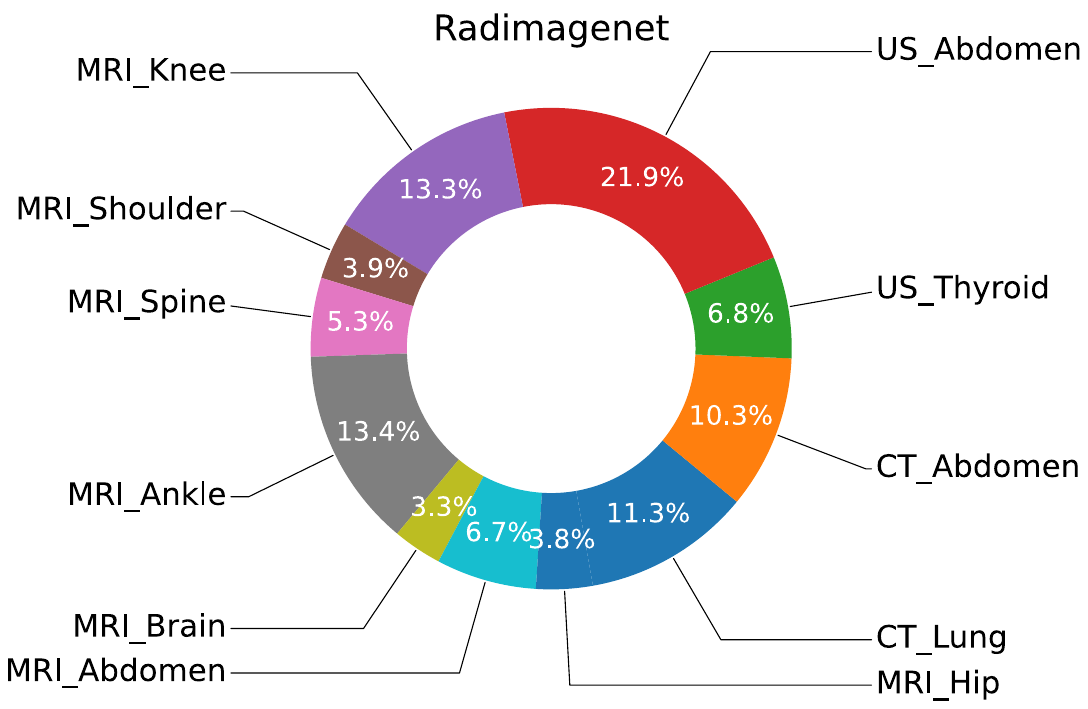}}
\end{minipage}
\hfill
\begin{minipage}{.48\linewidth}
\resizebox{1.12\textwidth}{!}{
\begin{tabular}{cccccc}
\multicolumn{6}{c}{\textbf{Radimagenet}}  \\
\toprule[1.5pt]
Task ID & Name & Modality & Region & Labels & Number  \\ \hline
1  & Lung  & CT   & Chest  & 6 & 152528 \\ \hline
2  & Abdomen  & CT & Abdomen & 28 & 139825\\ \hline
3  & Thyroid  & Ultrasound & Neck & 2 & 92599   \\ \hline
4  & Abdomen  & Ultrasound  &  Abdomen  & 13  & 297286   \\ \hline
5  & Knee  & MRI  &  Knee  & 18 & 179555 \\ \hline
6  & Shoulder &  MRI & Shoulder   & 14 &  52407\\ \hline
7  &  Spine& MRI  & Spine   & 9 &71674  \\ \hline
8  & Ankle &MRI  & Foot   & 25 & 181603 \\ \hline
9  & Abdomen &  MRI & Abdomen   & 26 & 91348 \\ \hline
10  & Brain &MRI   &  Head  & 10 & 44671 \\ \hline
11  & Hip &  MRI &  Hip  & 14 &  51417\\ 
\bottomrule[1.5pt]
\end{tabular}}
\end{minipage}
\caption{...}
\label{zrotate}
\end{figure*}

\begin{figure*}[h]
\begin{minipage}{0.48\linewidth}
 \centerline{\includegraphics[width=0.98\linewidth]{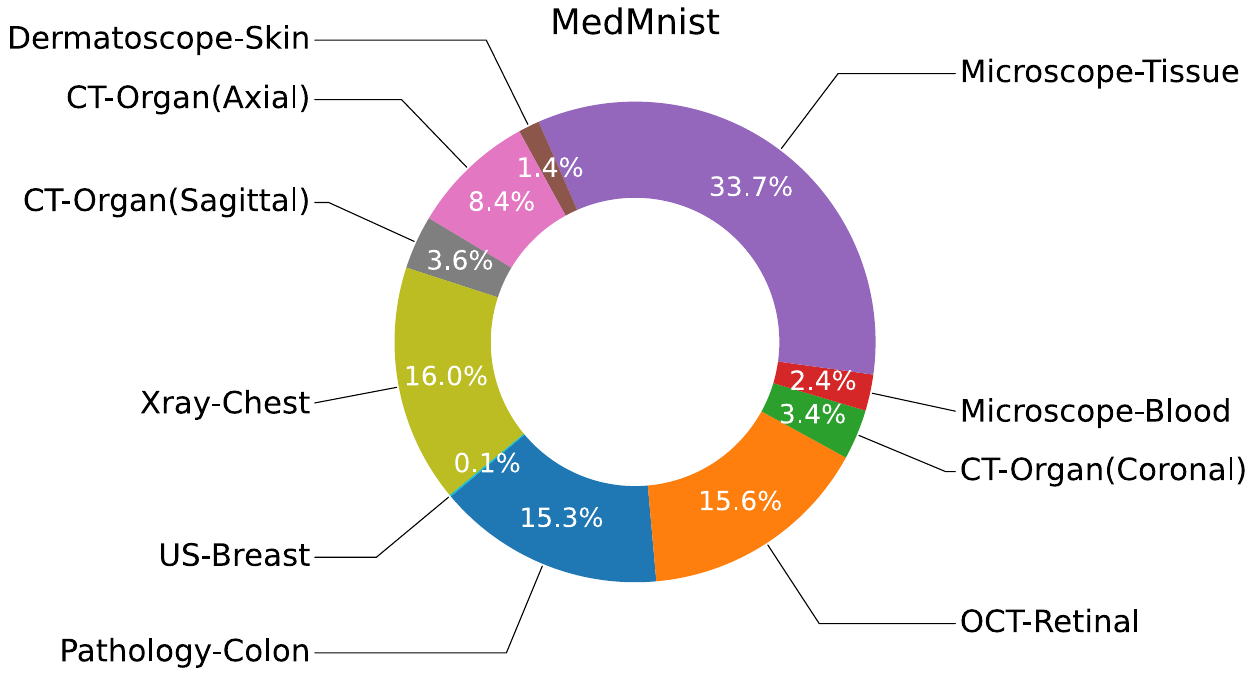}}
\end{minipage}
\hfill
\begin{minipage}{.48\linewidth}
\resizebox{1.12\textwidth}{!}{
\begin{tabular}{cccccc}
\multicolumn{6}{c}{\textbf{MedMnist}}  \\
\toprule[1.5pt]
Task ID & Name & Modality & Region & Labels & Number  \\ \hline
1  & Colon  & Pathology   & Colon  & 9  & 107180  \\ \hline
2  & Retinal  & OCT & Eye & 4 & 109309  \\ \hline
3  & OrganC  & CT & Abdomen & 11 & 23660   \\ \hline
4  & Cell  & Microscope  &  Blood  & 8  & 17092   \\ \hline
5  & Breast  & Ultrasound  &  Breast  & 2 & 780 \\ \hline
6  & Tissue & Microscope  &  Kidney cortex  & 8 & 236386 \\ \hline
7  & Skin & Dermatoscope  &  Skin  & 7 & 10015 \\ \hline
8  & OrganA  & CT  &  Abdomen  & 11 & 58850 \\ \hline
9  & OrganS & CT  &  Abdomen  & 11 & 25221 \\ \hline
10  & Chest & Xray  &  Chest  & 2 &  112120 \\ 
\bottomrule[1.5pt]
\end{tabular}}
\end{minipage}
\caption{...}
\label{zrotate}
\end{figure*}

\begin{figure*}[h]
\begin{minipage}{0.48\linewidth}
 \centerline{\includegraphics[width=0.98\linewidth]{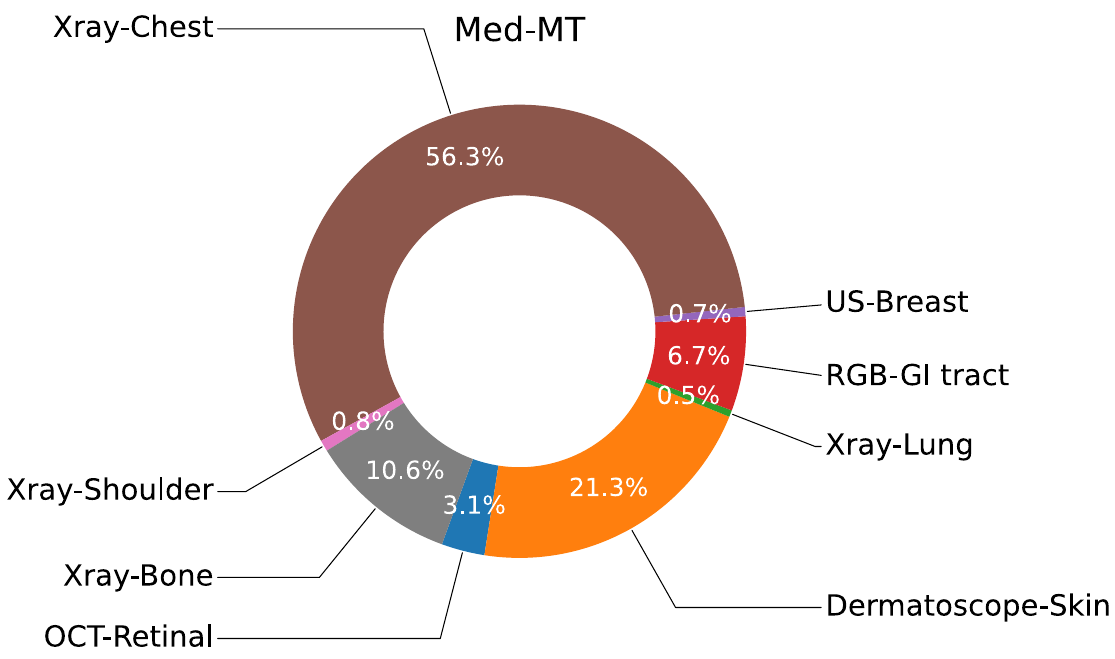}}
\end{minipage}
\hfill
\begin{minipage}{.48\linewidth}
\resizebox{1.12\textwidth}{!}{
\begin{tabular}{cccccc}
\multicolumn{6}{c}{\textbf{Med-MT}}  \\
\toprule[1.5pt]
Task ID & Name & Modality & Region & Labels & Number  \\ \hline
1  & Retinal  & OCT   & Eye  & 5  & 3662  \\ \hline
2  & Skin  & Dermatoscope & Skin & 3 & 25331  \\ \hline
3  & Breast  & Ultrasound & Breast & 8 & 780   \\ \hline
4  & GI tract  & RGB  &  Gastrointestinal  & 8  & 8000   \\ \hline
5  & Lung  & Xray  &  Chest  & 2 & 566 \\ \hline
6  & Shoulder &  Xray &   Shoulder & 4 & 945 \\ \hline
7  & Lung &  Xray &   Chest & 15 &  67914 \\ \hline
8  & Bone &  Xray &  Bone  & 12 & 12611 \\ 
\bottomrule[1.5pt]
\end{tabular}}
\end{minipage}
\caption{...}
\label{zrotate}
\end{figure*}

\begin{table}[h]
\caption{Overview of downstream medical datasets.}
\resizebox{0.48\textwidth}{!}{
\begin{tabular}{cccccc}
\toprule[1.5pt]
Task ID & Name & Modality & Region & Labels & Number  \\ \hline
1  & COVID  & CT   & Chest  & 2  & 746  \\ \hline
2  & BTC  & MRI & Head & 4 & 3538  \\ \hline
3  & AD  & MRI & Head & 4 & 3264   \\ \hline
4  & Mura\_shoulder  & MRI  &  Shoulder  & 2  & 8942   \\ \hline
5  & AUTID  & Ultrasound  &  Neck  & 3 & 6400 \\ \hline
6  & HAM10000 & Dermatoscope  &  Skin  & 7 &  10015\\ \hline
7  & DET10 &  Xray & Chest   & 10 & 3543 \\ 
\bottomrule[1.5pt]
\end{tabular}}
\label{dataset-tab}
\end{table}

\begin{table*}[h]
\caption{Overview of downstream medical datasets.}
\resizebox{1.06\textwidth}{!}{
\setlength{\tabcolsep}{5.8mm}{
\begin{tabular}{c|ccccccc}
\toprule[1.5pt]
Pre-trained & COVID & BTC & AD & Mura\_s & AUTID & HAM10000 & DET10  \\ \hline
Radimagenet  & Expert\_1  &  Expert\_10 & Expert\_10  & Expert\_6 &  Expert\_3 & Expert${^\dagger}$ & Expert\_1\\ \hline
MedMnist  & Expert\_10  & Expert${^\dagger}$ & Expert${^\dagger}$  & Expert${^\dagger}$ & Expert\_5  & Expert\_7 & Expert\_10  \\ \hline
Med-MT   &  Expert${^\dagger}$ & Expert${^\dagger}$ & Expert${^\dagger}$  & Expert${^\dagger}$ & Expert${^\dagger}$  & Expert\_2 & Expert${^\dagger}$ \\ 
\bottomrule[1.5pt]
\end{tabular}}}
\label{dataset-tab}
\end{table*}
